# Supplementary material for: Chemical Reaction Dynamics under Vibrational Strong Coupling
Source: arXiv:2402.04256 source file (2024-01-03)
Supplement: Supplementary file 1 [file appendix-1.tex]

\begin{savequote}[8cm]
The heart of animals is the foundation of their life, the sovereign of everything within them, the sun of their microcosm, that upon which all growth depends, from which all power proceeds.
  \qauthor{--- William Harvey \cite{harvey_exercitatio_1628}}
\end{savequote}

\chapter{\label{app:1-}Review of Cardiac Physiology and Electrophysiology}

\minitoc

Appendices are just like chapters.  Their sections and subsections get numbered and included in the table of contents; figures and equations a

\section{Mechanical Cycle}

Sed iaculis faucibus odio, eu aliquam purus efficitur vel. Cras at nulla ac enim congue varius ut et nulla. Integer blandit mattis augue.

\section{Electrical Cycle}
\label{sec:electcycle}

Lo

\section{Cellular Electromechanical Coupling}
\label{sec:electromech}

Nunc volutpat efficitur lacus in aliquet. Nullam non iaculis diam, at ultrices diam. Proin vehicula vulputate cursus. Morbi tempus sapien id urna lobortis interdum. Maecenas elementum sagittis elementum. Donec at sodales velit, a posuere tortor. Nulla id hendrerit tortor. Sed semper velit in magna sagittis pulvinar. Nulla nec arcu molestie, ultricies sapien sit amet, sollicitudin nisi. Donec nisi massa, suscipit ut dignissim quis, lacinia id leo.

Suspendisse ut mi metus. Morbi tincidunt ligula in porttitor consectetur. Integer eu urna urna. Suspendisse potenti. Mauris sit amet felis eu diam auctor ullamcorper. Morbi in porta nisi. Nam ante tortor, venenatis vitae tempor sed, sagittis vitae velit. In semper orci sit amet nisi ullamcorper varius. Aenean dignissim ultrices imperdiet. Maecenas lacinia enim id neque porttitor iaculis. Curabitur laoreet ante ut urna dignissim, id sollicitudin metus consectetur. Aenean massa ipsum, auctor vel ante vel, blandit dignissim libero. Fusce interdum ac magna et interdum.
